# Supplementary material for: Deterministic Memory Abstraction and Supporting Multicore System Architecture
Source: arXiv:1707.05260 source file (2018-04-19)
Supplement: Supplementary file 1 [file appendix.tex]

\subsection{Additional Results for Best-effort Tasks} \label{subsec:ext-best-effort}

\begin{figure} [h]
    \centering
    \begin{subfigure}{0.48\textwidth}
        \includegraphics[width=\linewidth]{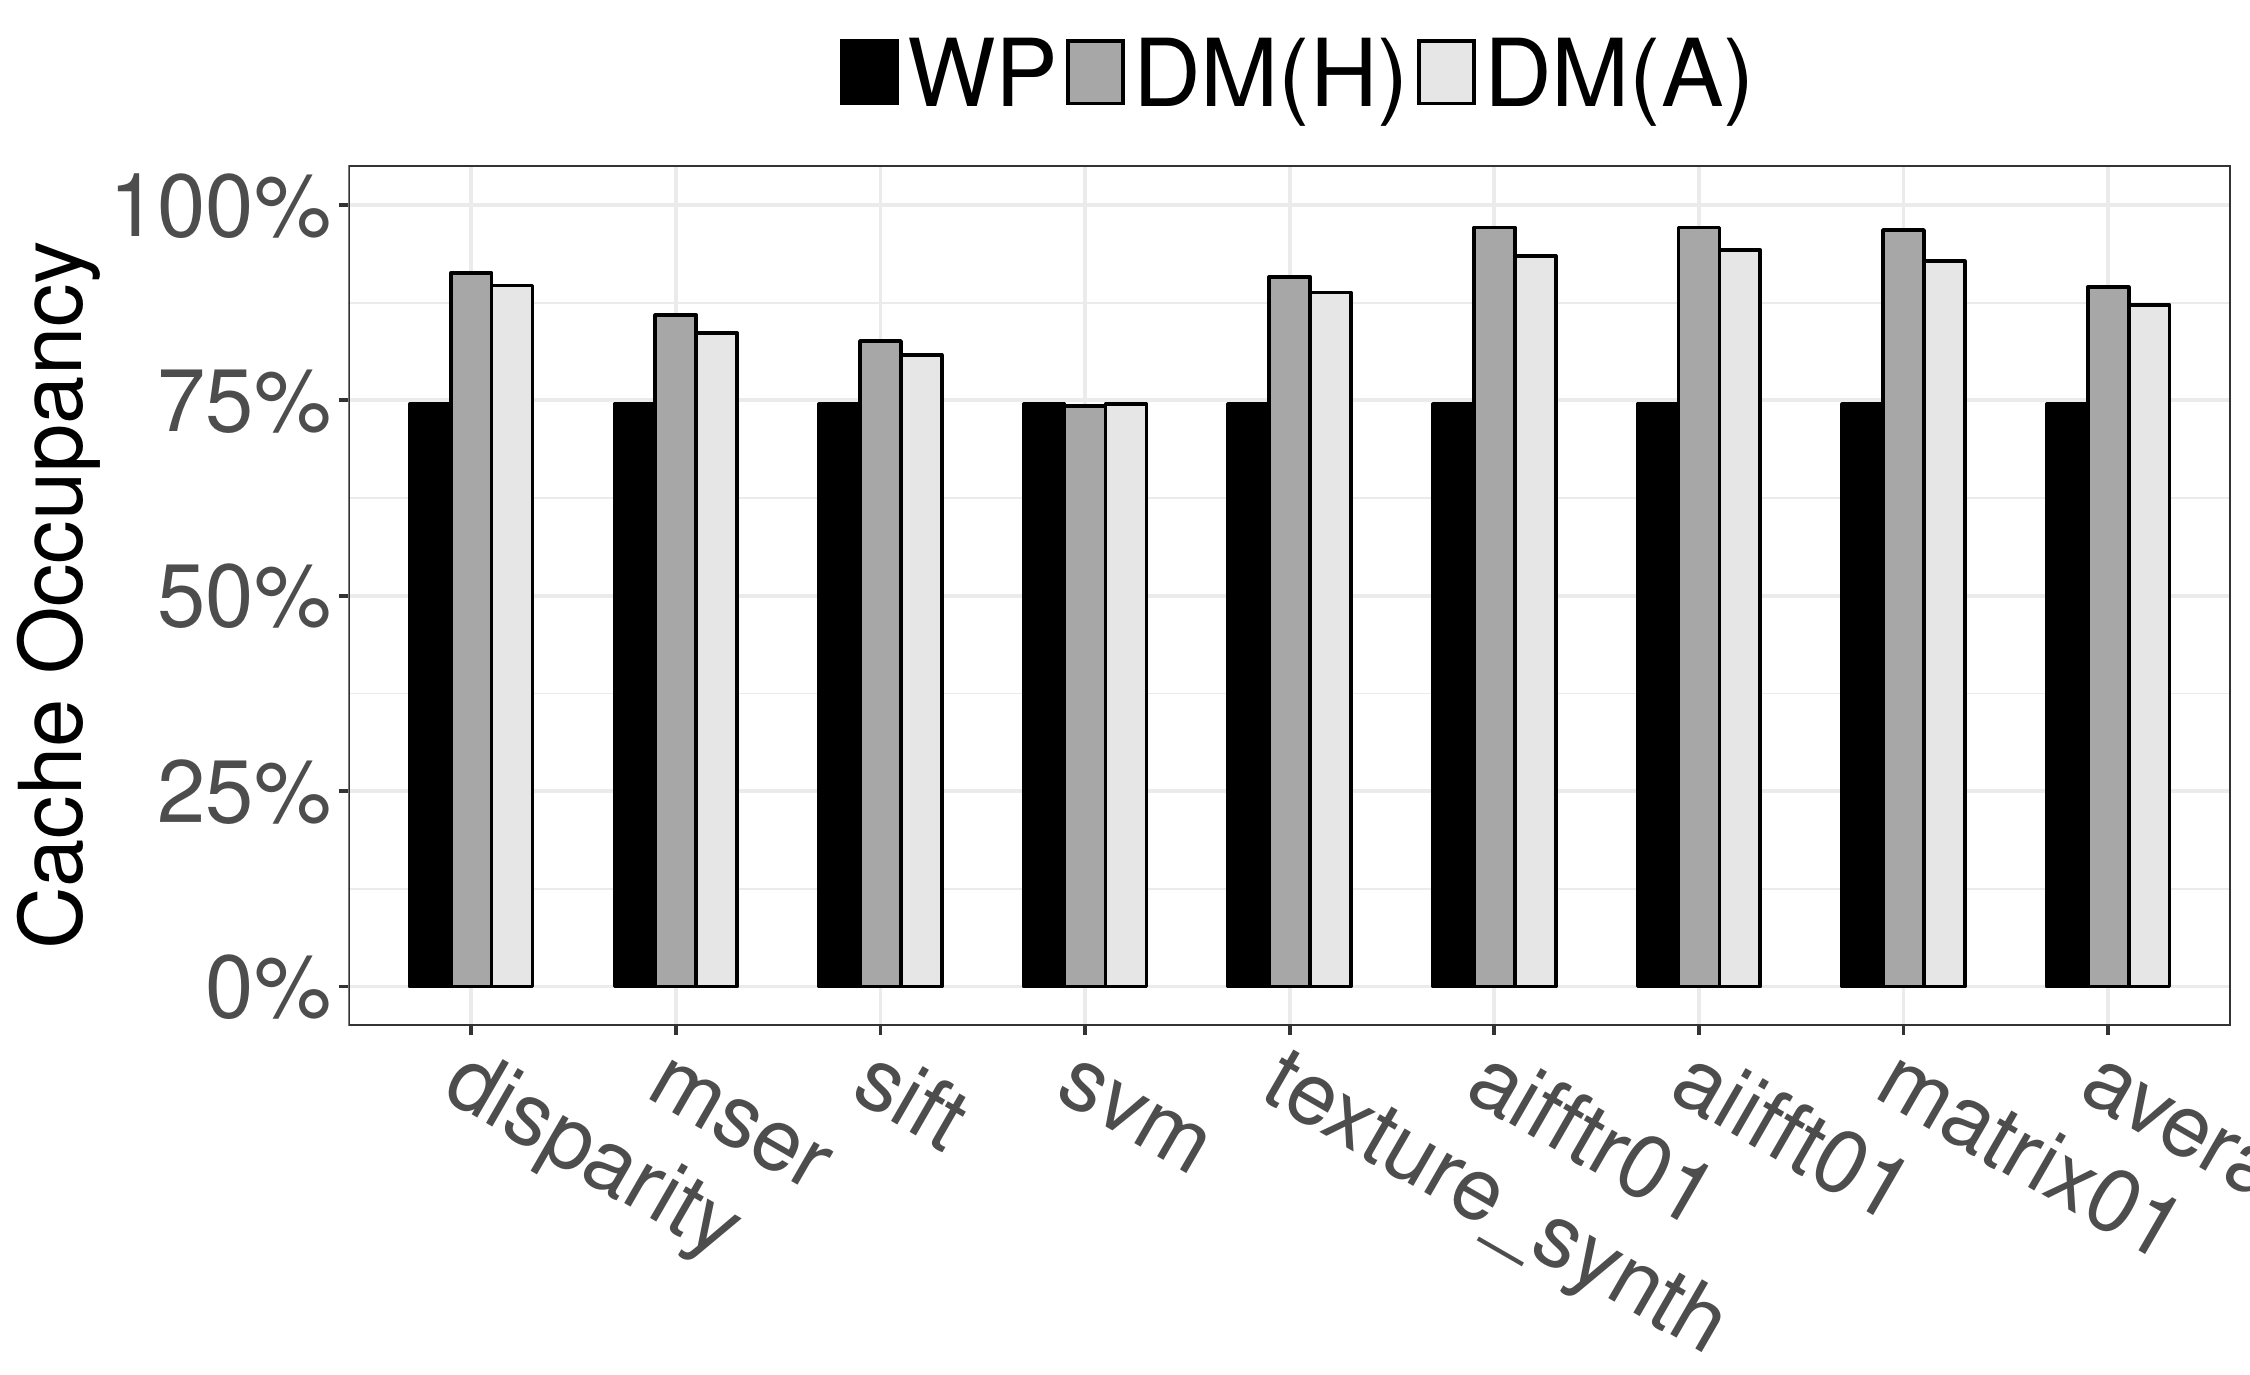}
        \caption{The percentage of total cache space occupied by \emph{bzip2} running on 3 cores.}
        \label{fig:bzip2-benefit2_a}
    \end{subfigure}
    \vfill
    \begin{subfigure}{0.48\textwidth}
        \includegraphics[width=\linewidth]{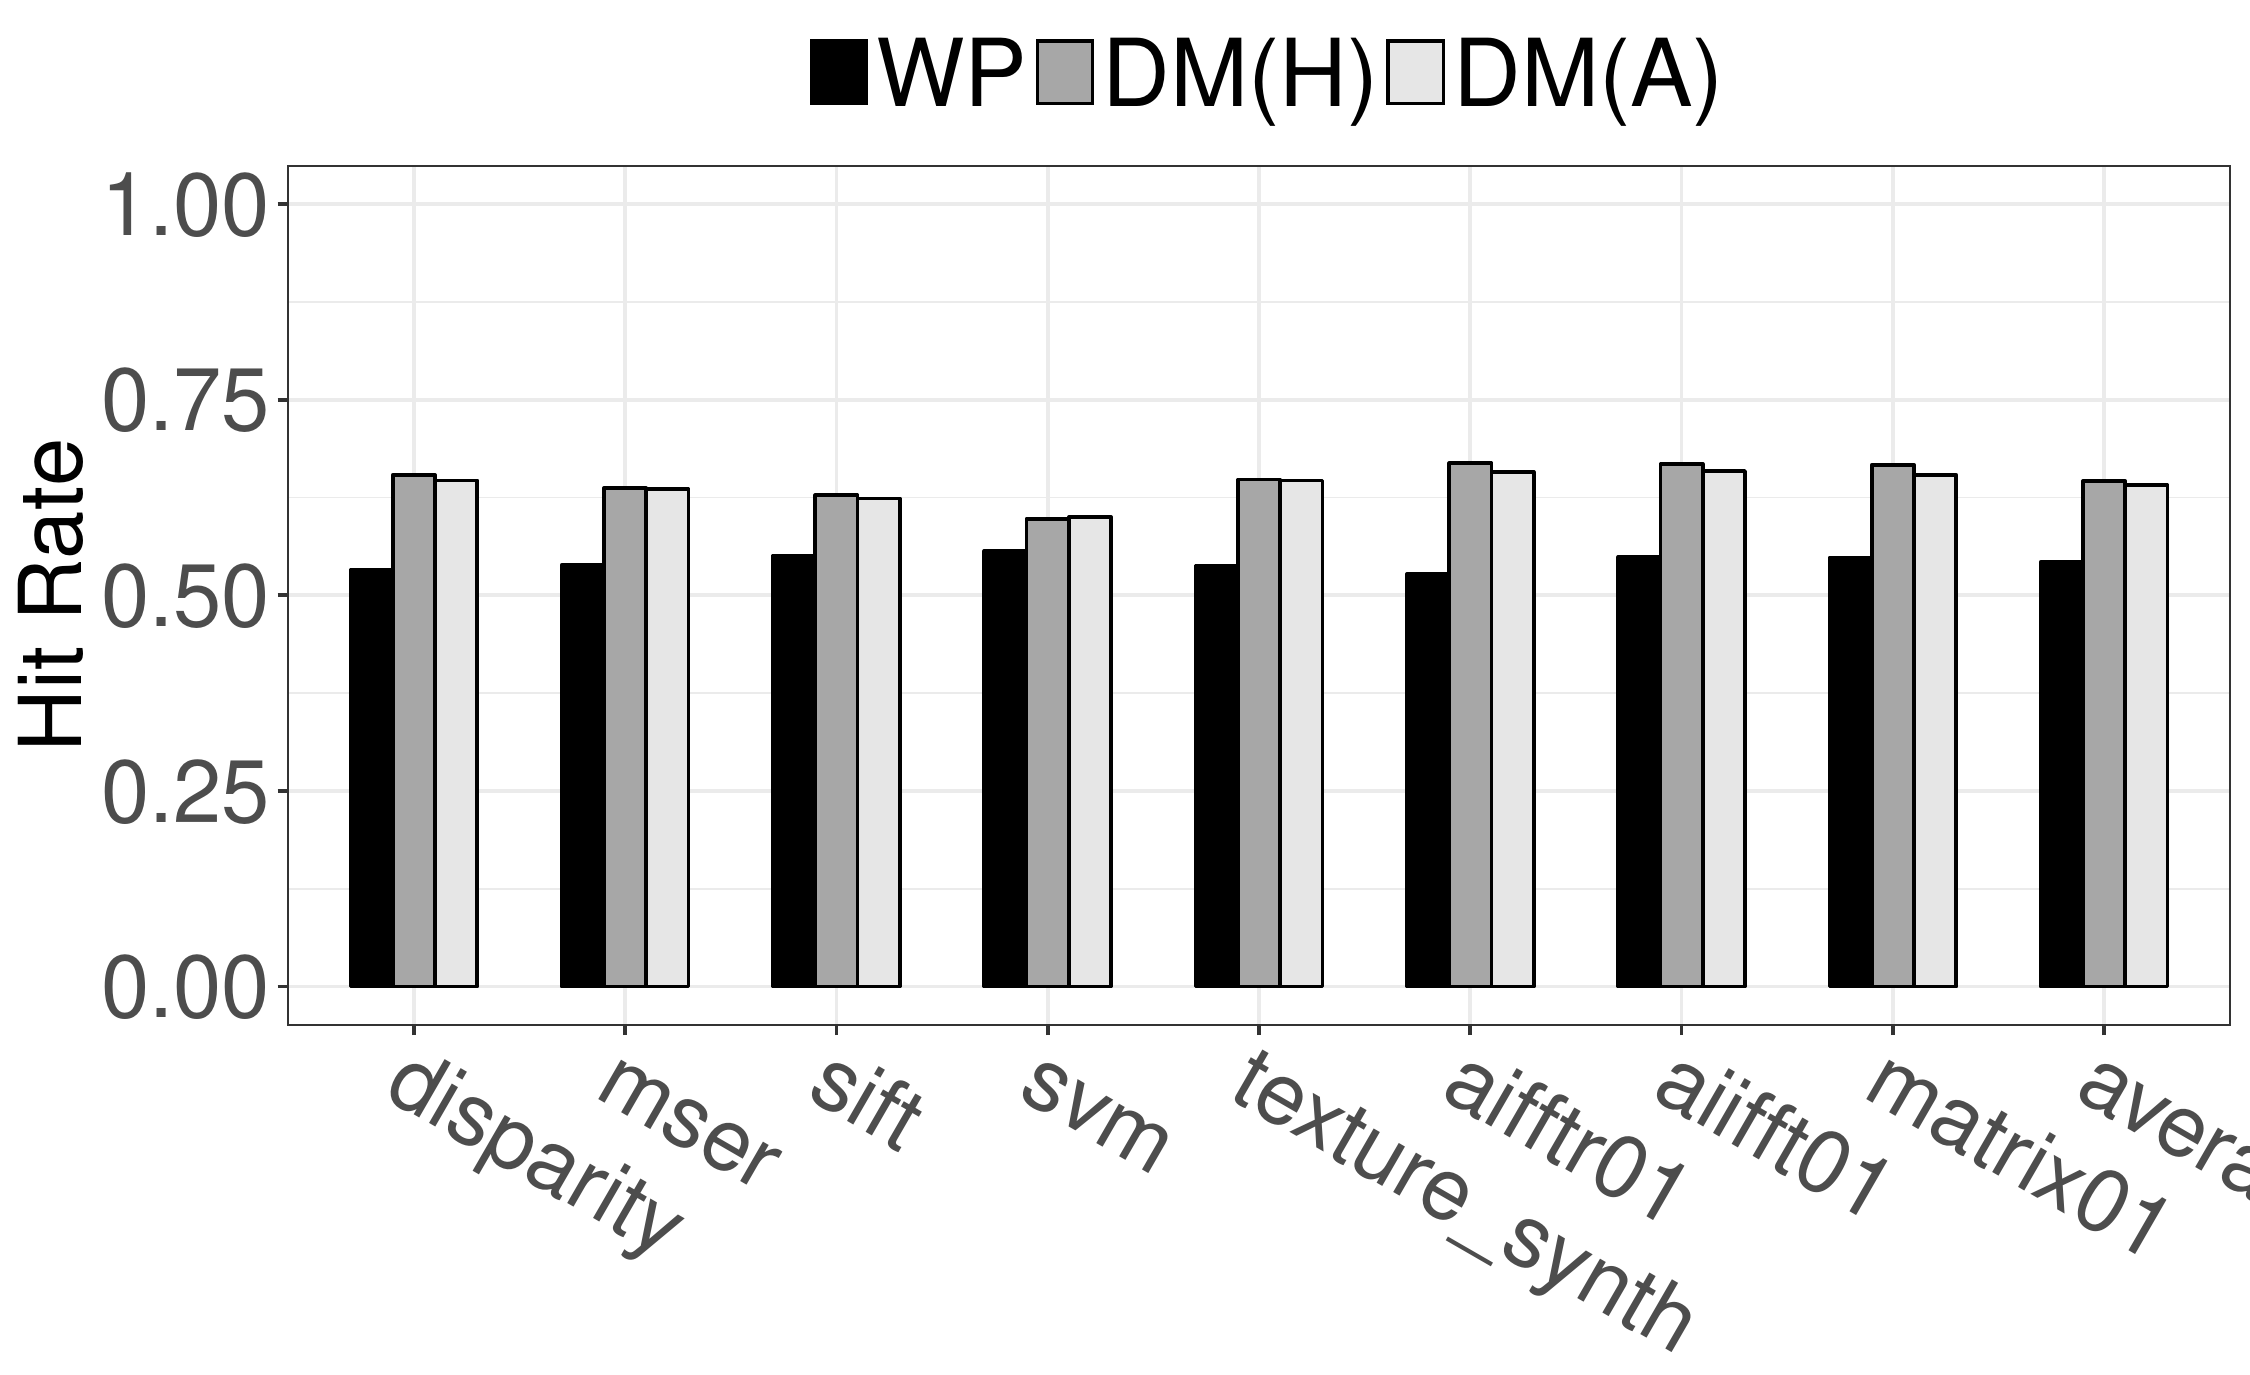}
        \caption{Average hit rate for \emph{bzip2} running on 3 cores.}
        \label{fig:bzip2-benefit2_b}
    \end{subfigure}

    \caption{Cache usage and hit rate of \emph{bzip2}.
    The real-time task is running Core 3, and
    three instances of \emph{bzip2} are running on Core 0 through 2.}
    \label{fig:bzip2-benefit2}
\end{figure}

\begin{figure} [h]
    \centering
    \begin{subfigure}{0.48\textwidth}
        \includegraphics[width=\linewidth]{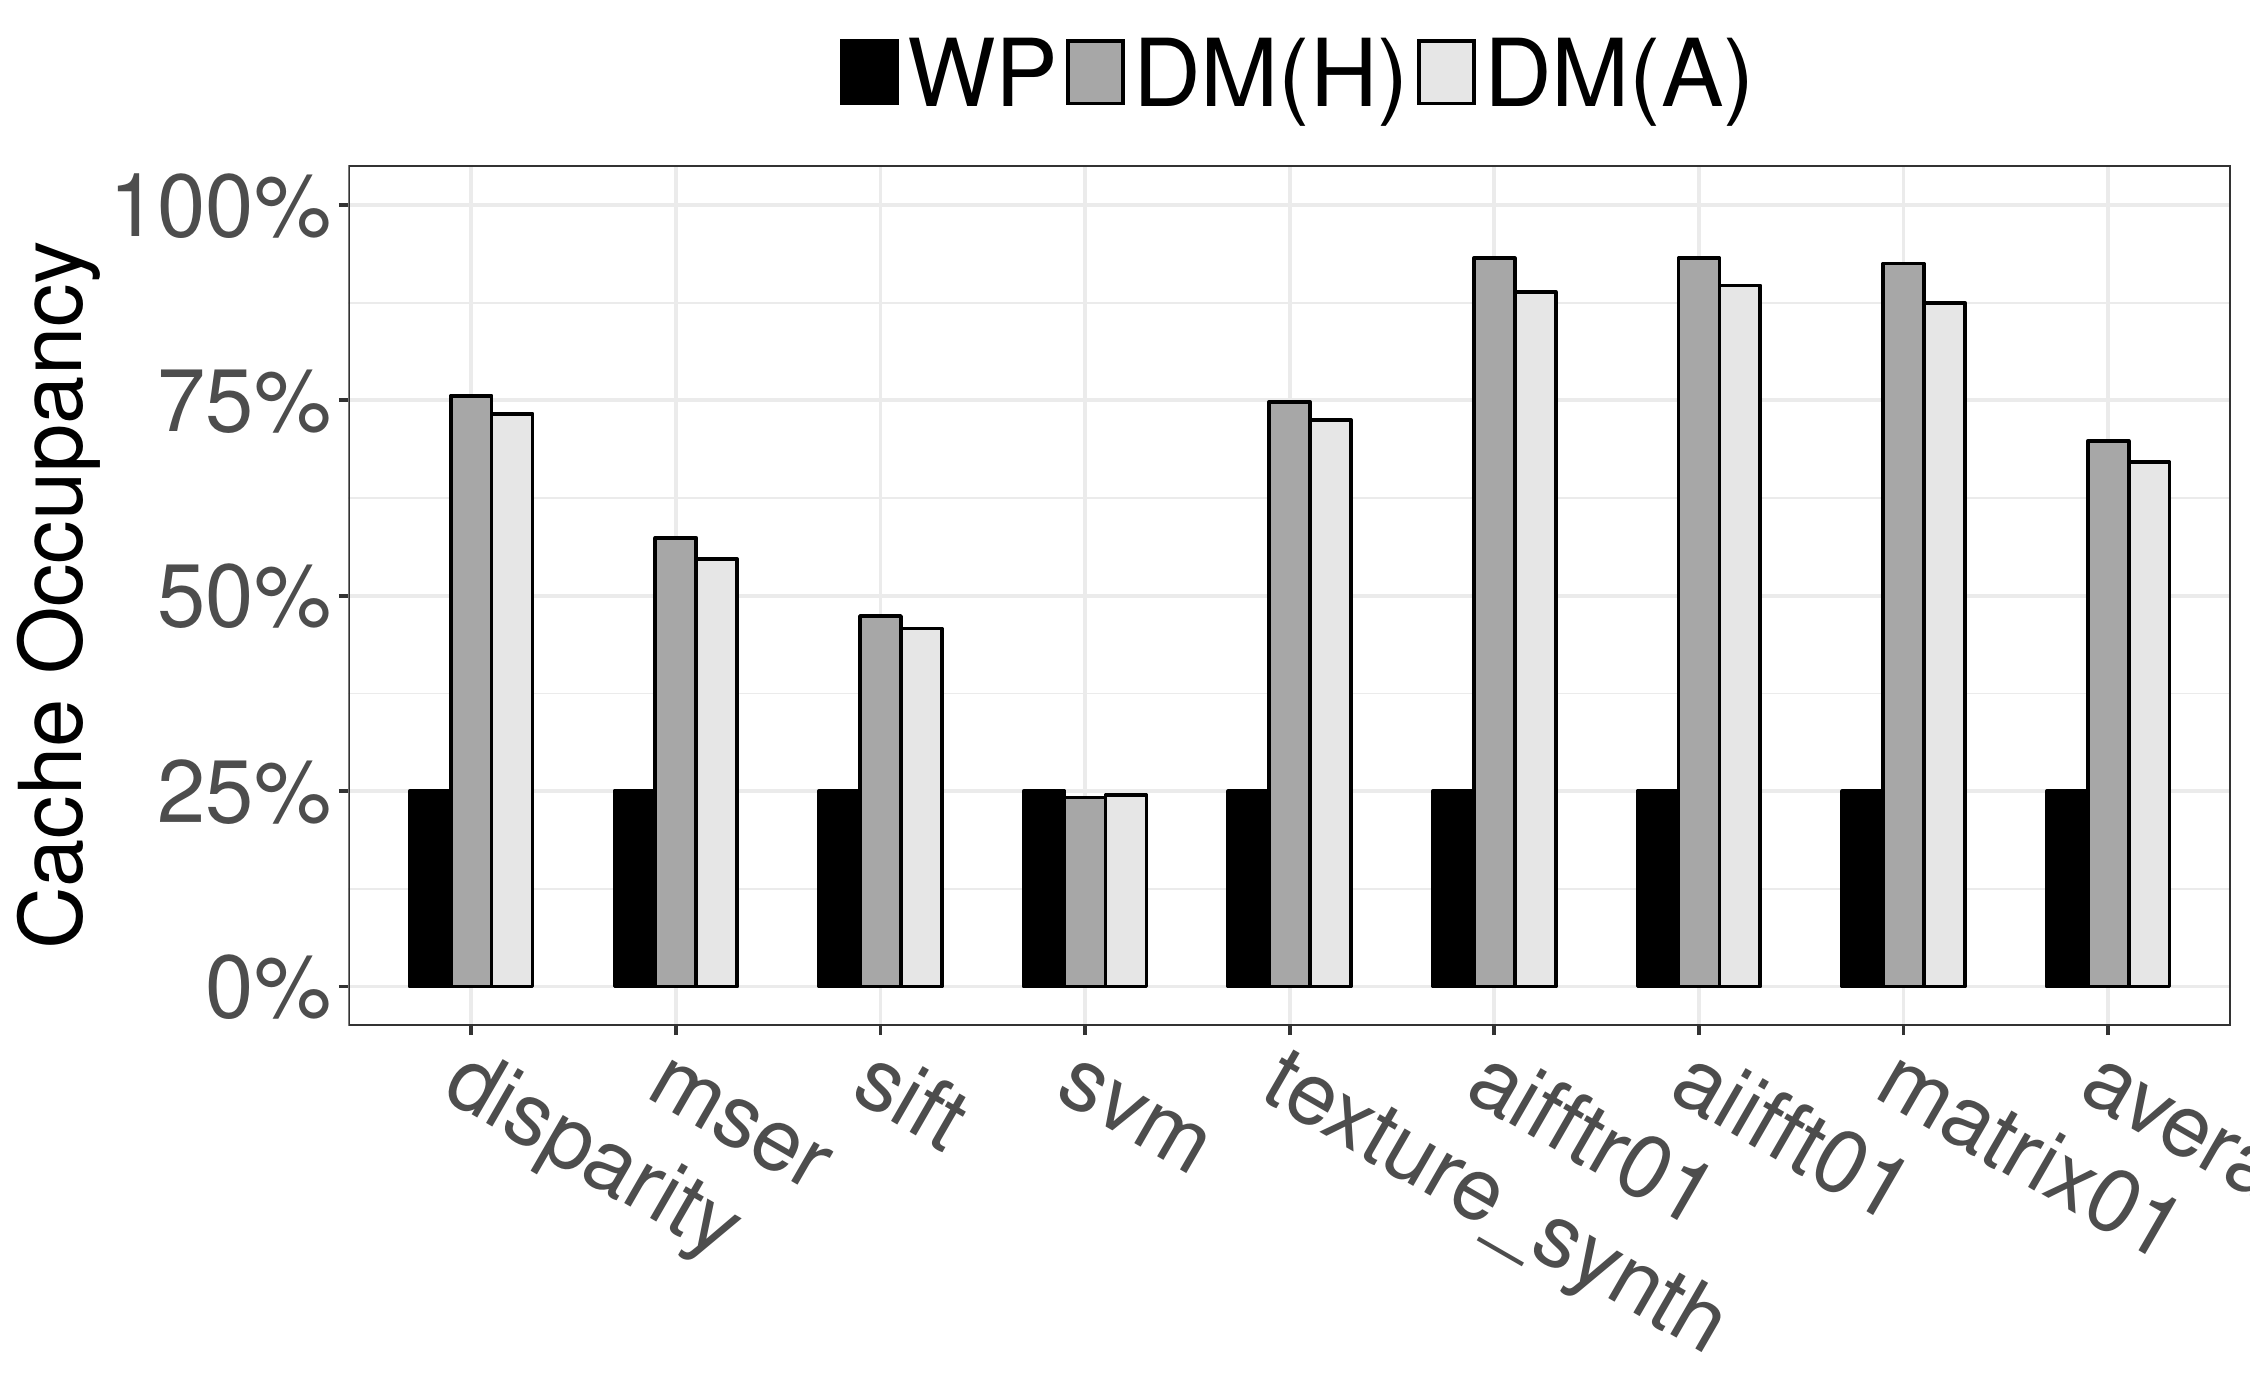}
        \caption{The percentage of cache space occupied by \emph{mcf}.}
    \end{subfigure}
    \hfill
    \begin{subfigure}{0.48\textwidth}
        \includegraphics[width=\linewidth]{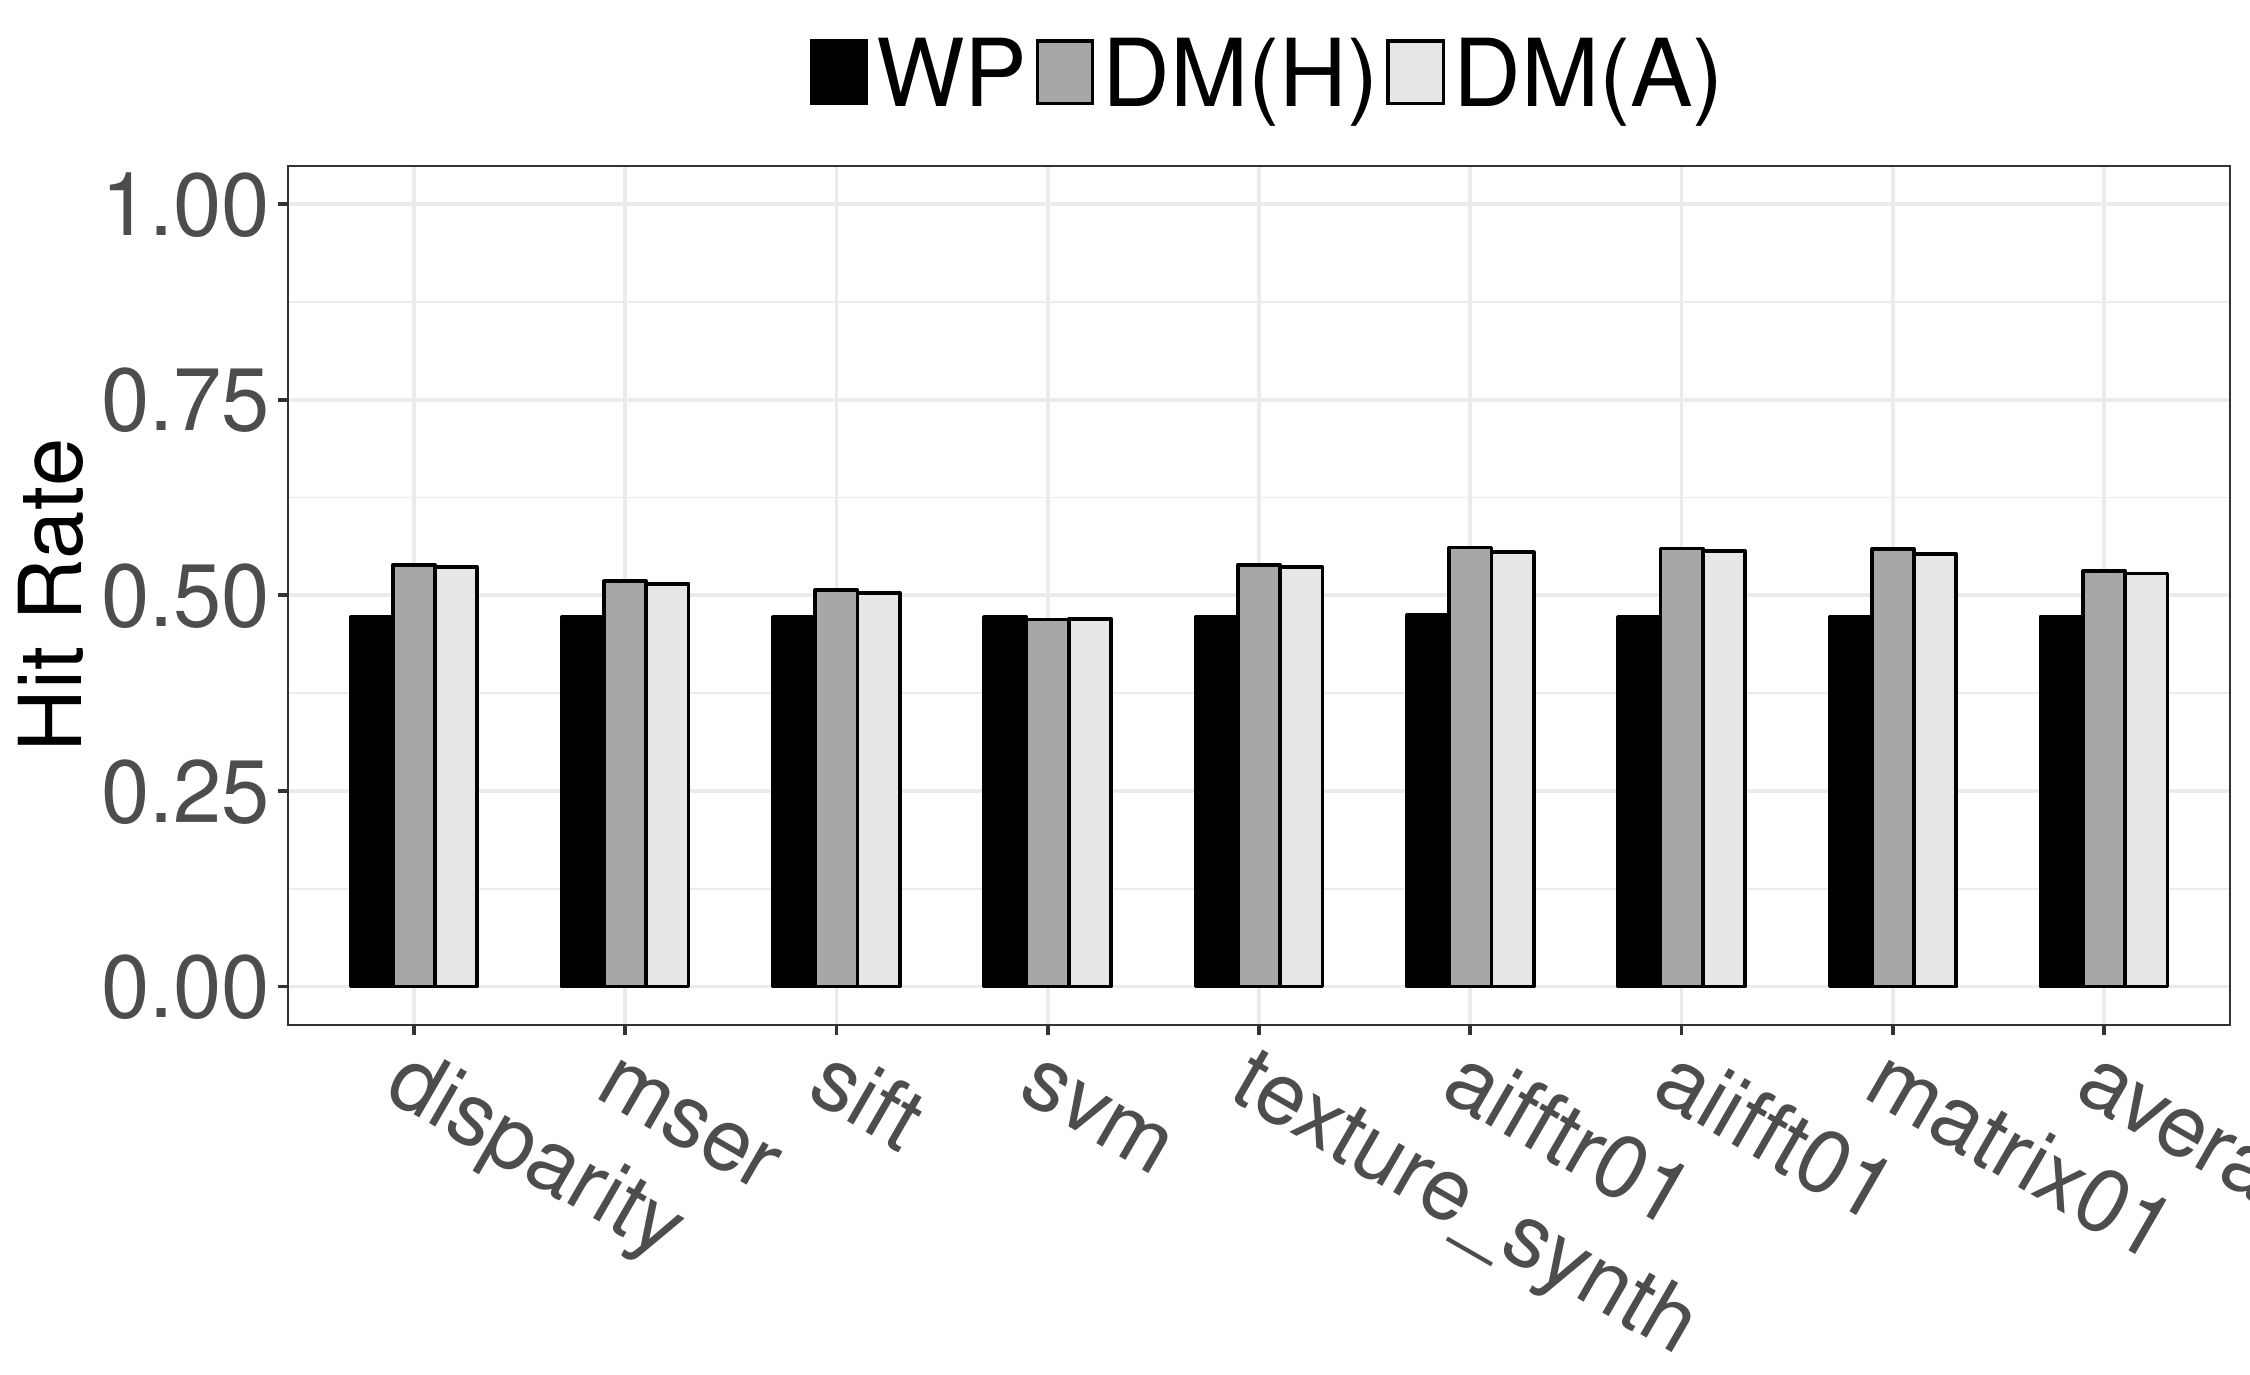}
        \caption{\emph{mcf} hit rate.}
    \end{subfigure}
    \vfill
    \begin{subfigure}{0.48\textwidth}
        \includegraphics[width=\linewidth]{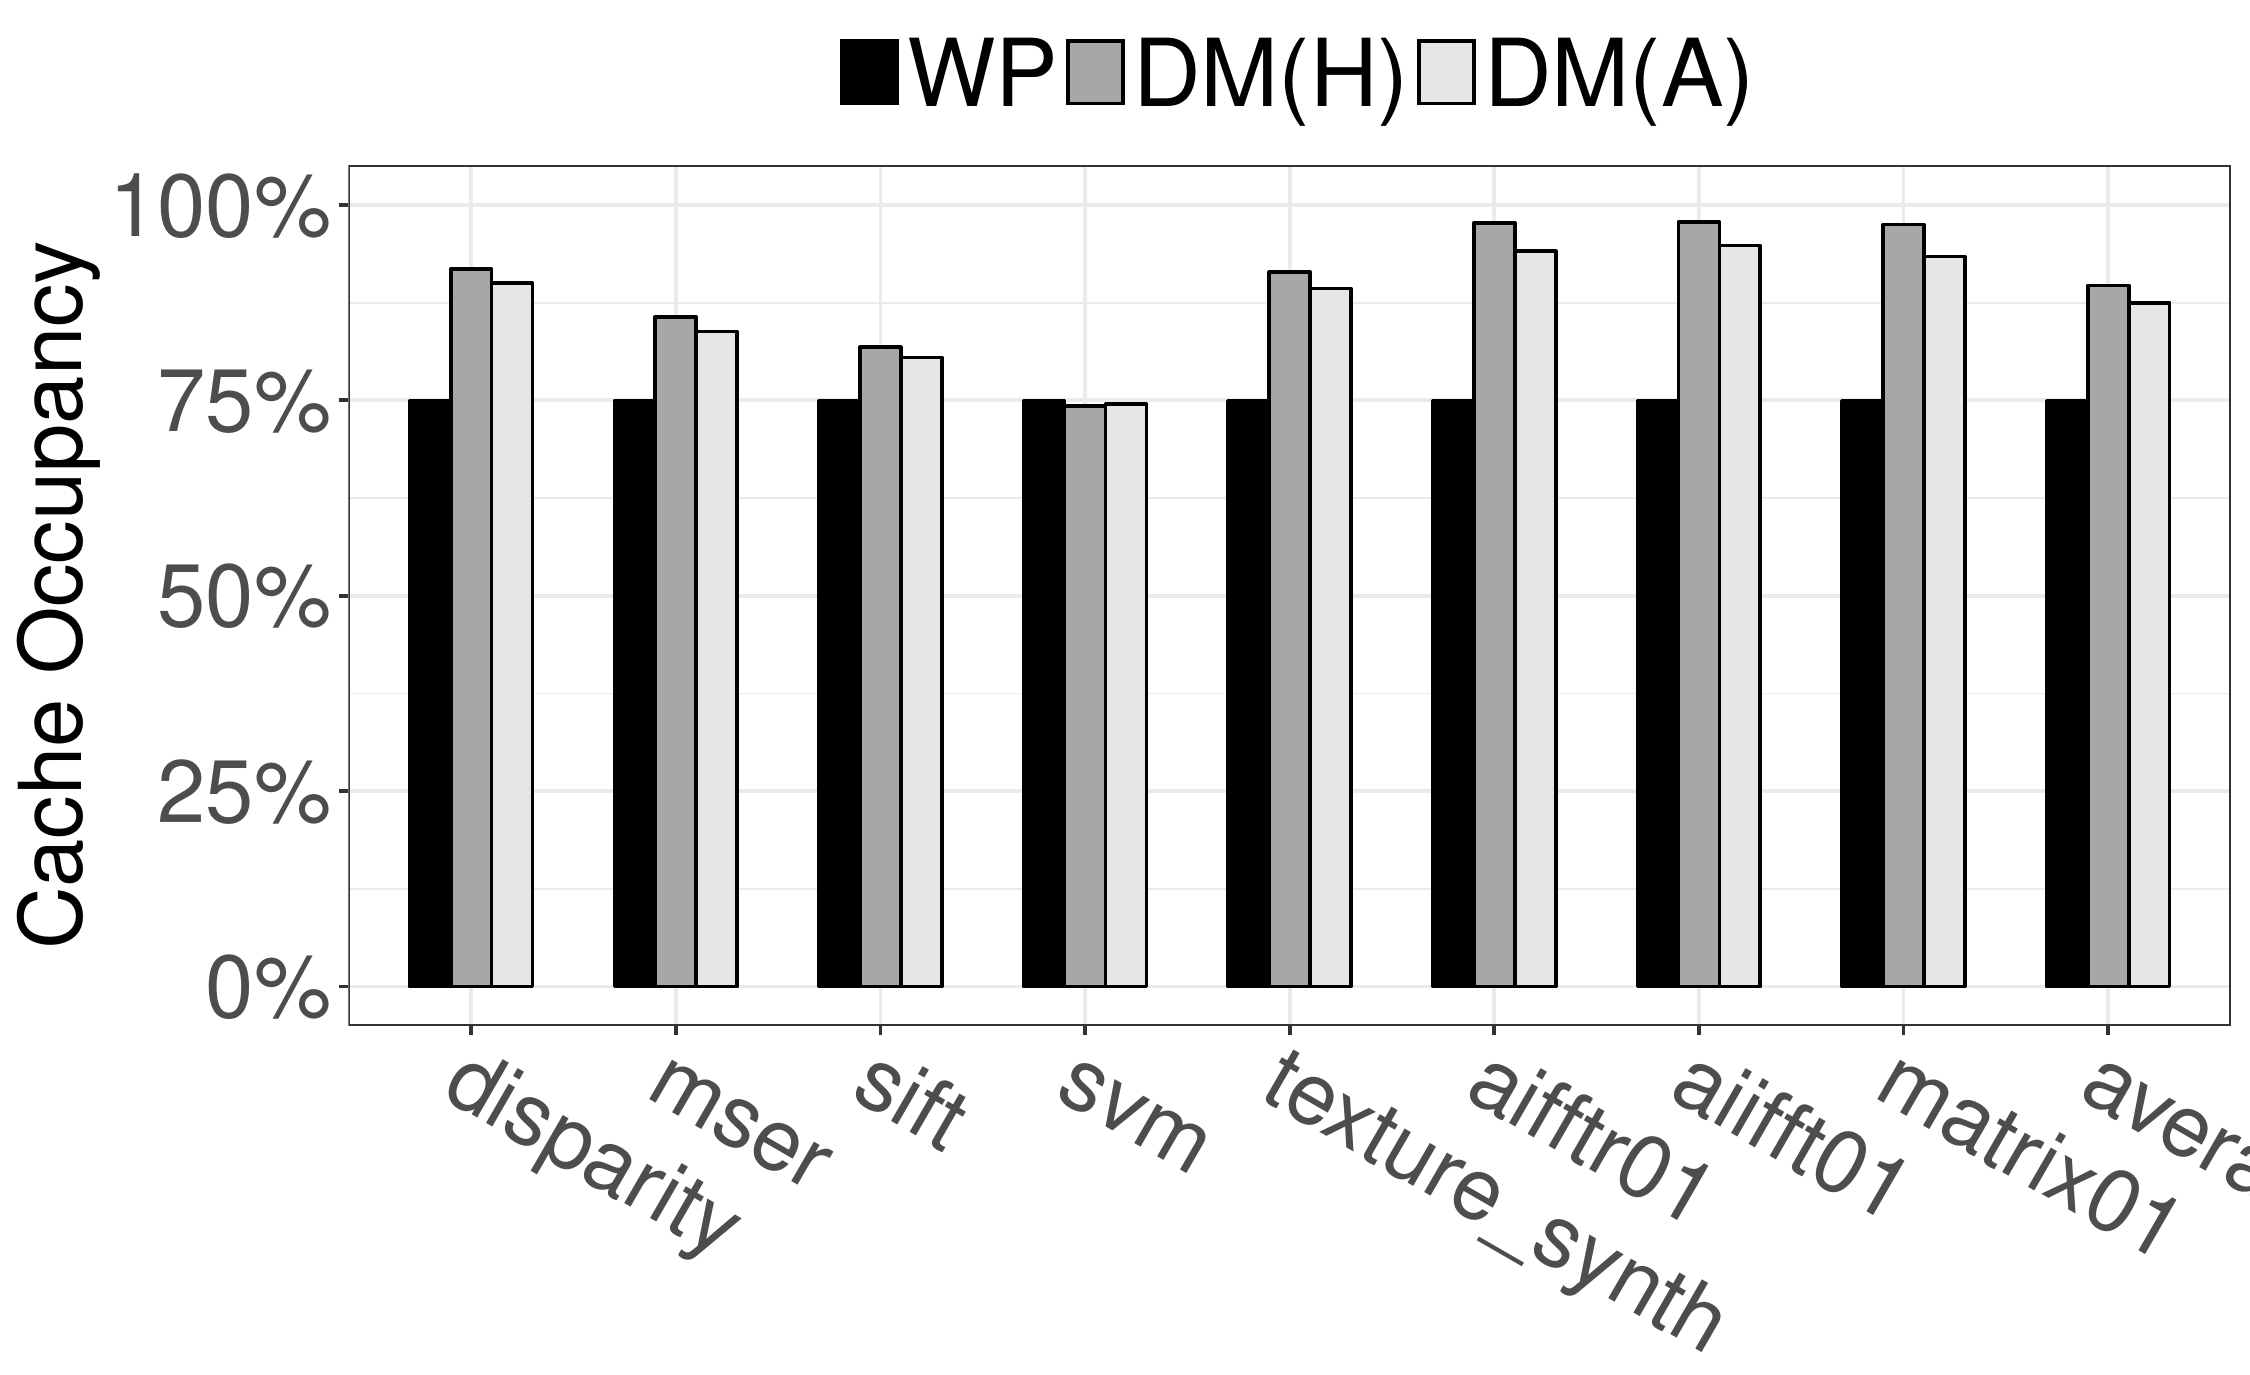}
        \caption{The percentage of total cache space occupied by \emph{mcf} running on 3 cores.}
    \end{subfigure}
    \hfill
    \begin{subfigure}{0.48\textwidth}
        \includegraphics[width=\linewidth]{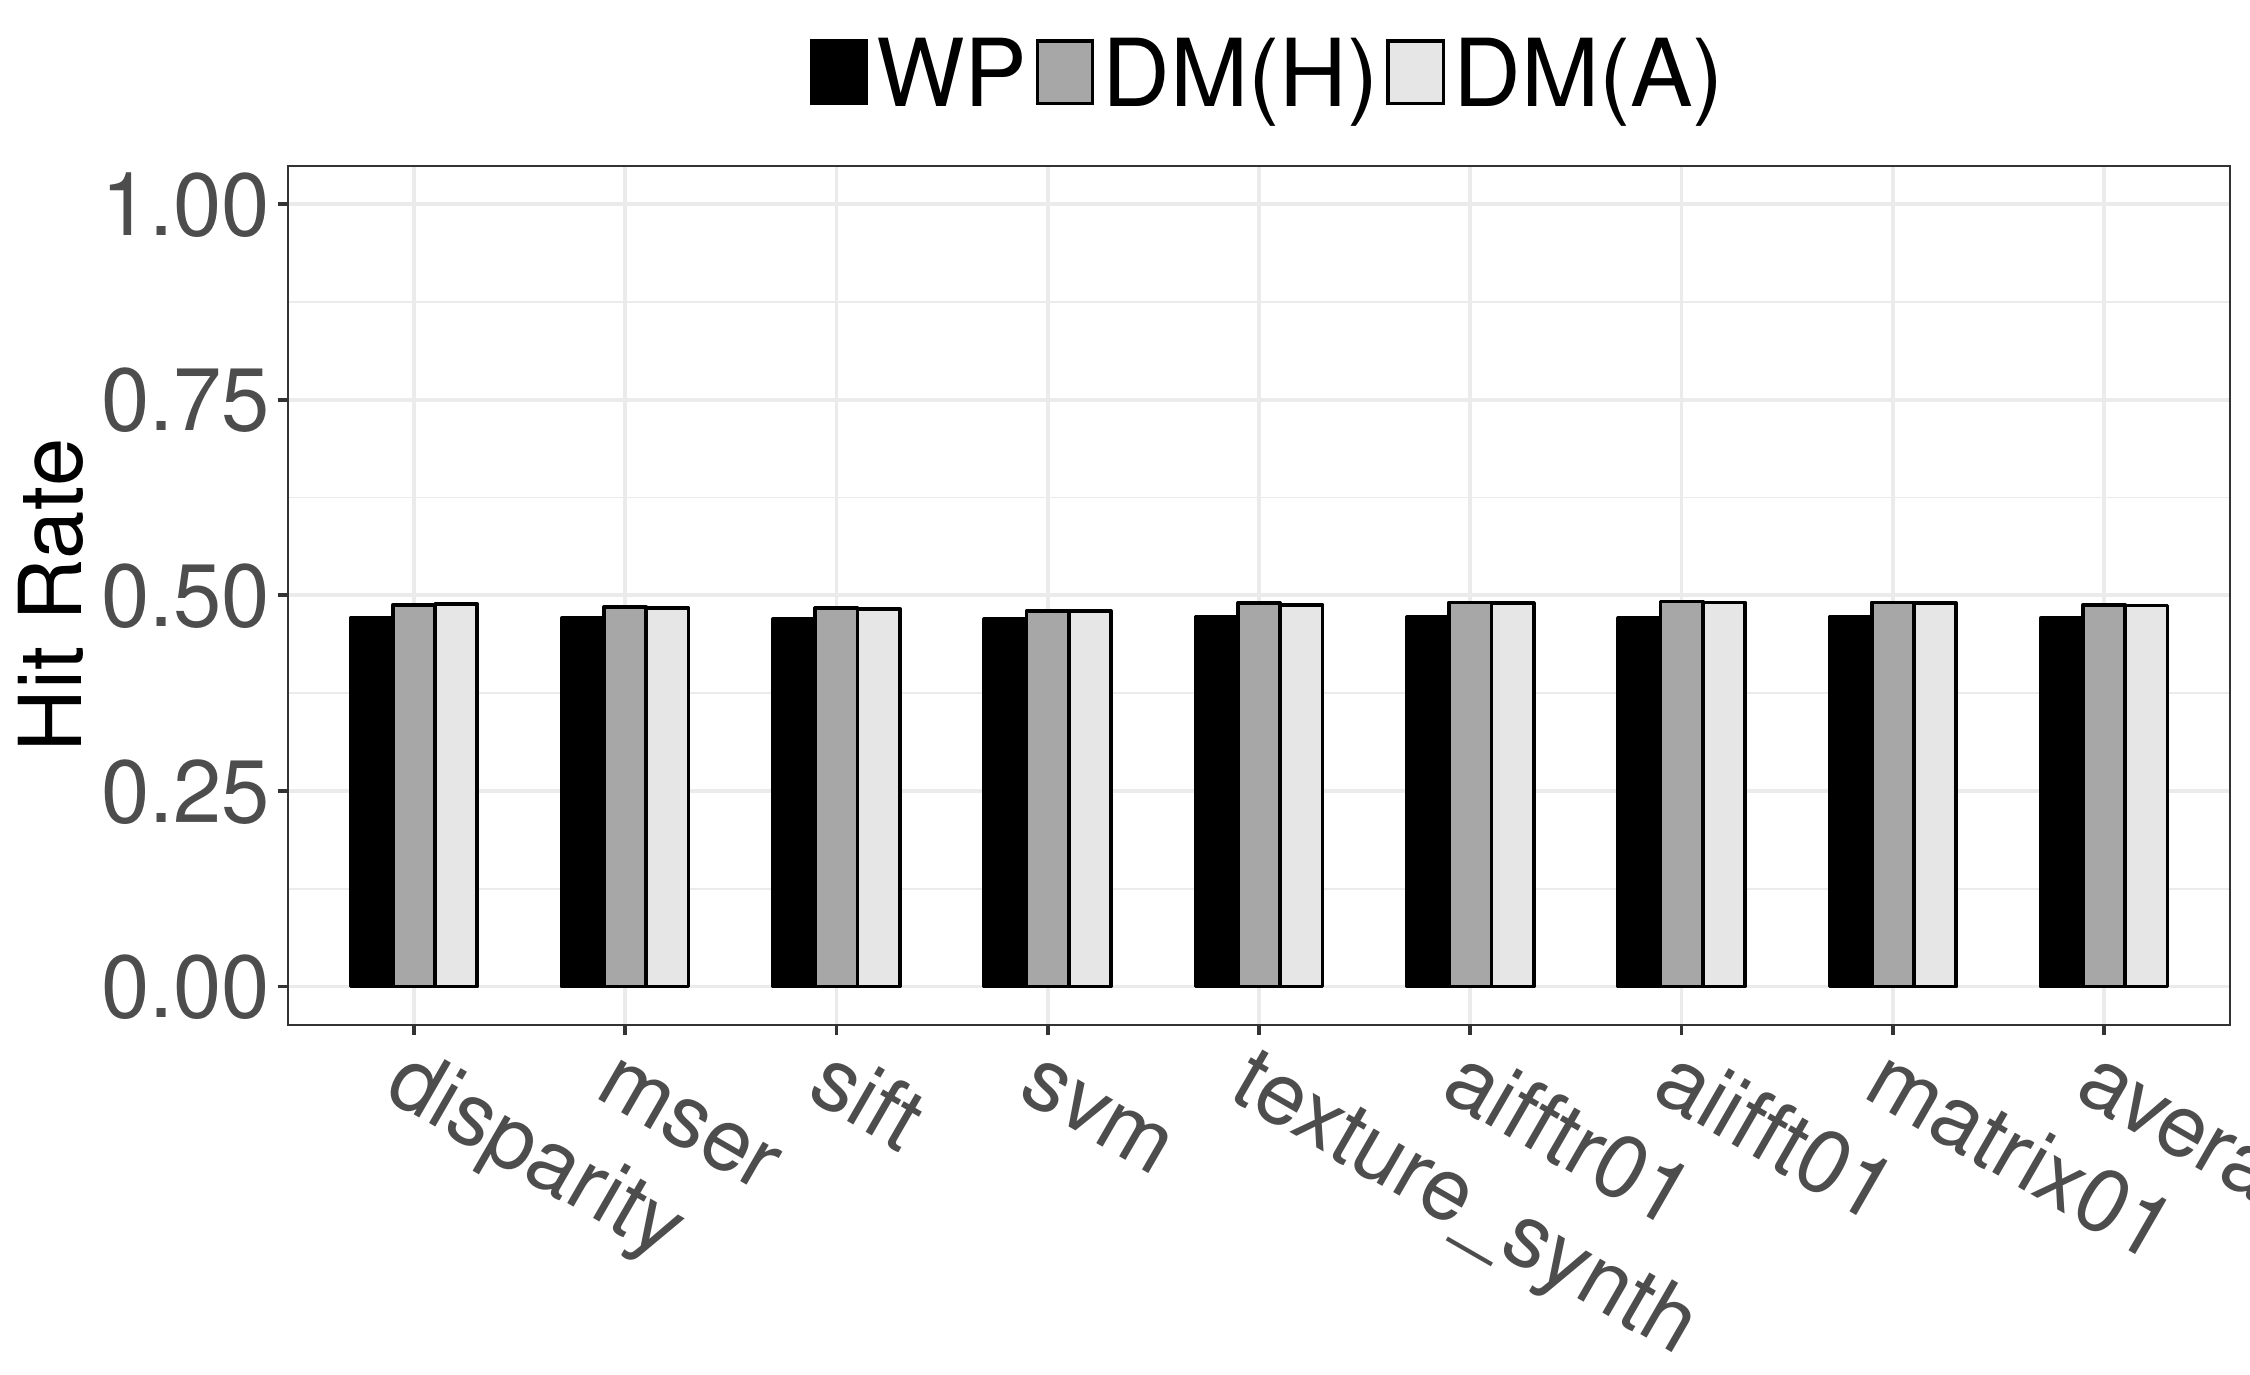}
        \caption{Average hit rate for \emph{mcf} running on 3 cores.}
    \end{subfigure}

    \caption{Cache usage and hit rate of \emph{mcf} for two
    different scenarios: 1) \emph{mcf} is running on one core, and 3 instances of the
    real-time task are running on rest of the cores (figures (a) and (b));
    2) the real-time task is running on one core, and three instances of 
    \emph{mcf} are running on the rest of the cores (figures (c) and (d)).}
    \label{fig:mcf-benefit}
\end{figure}

Figure~\ref{fig:bzip2-benefit2_a} shows the result for Scenario~2
(see \ref{subsec:best-effort}).
As it can bee seen, three instances of bzip2 occupy 75\% of
cache space in WP (each gets 25\%). To calculate the cache space each
\emph{bzip2} occupies in DM(H) and DM(A), the numbers in
Figure~\ref{fig:bzip2-benefit2_a} must be divided by 3.
By doing this calculation, we can see that each \emph{bzip2}
occupies less cache space compared to what has been observed in Scenario~1
(Figure \ref{fig:bzip2-benefit_a}). This results in a smaller hit rate improvement 
compared to Scenario~1, as can be observed by comparing Figure~\ref{fig:bzip2-benefit_b} 
and Figure~\ref{fig:bzip2-benefit2_b}.

Figure~\ref{fig:mcf-benefit} shows the result for \emph{mcf}. By comparing
this figure to figures \ref{fig:bzip2-benefit} and \ref{fig:bzip2-benefit2},
we can observe that the amount of cache space that \emph{mcf} and \emph{bzip2}
are allowed to occupy is the same. This means that, although cache space occupation 
increase from WP to DM(H) or DM(A) is the same
for both benchmarks, \emph{bzip2} benefits more from the additional space in terms of hit rate.

\section{LRU Persistence Analysis under Deterministic Memory}

In this section we provide a sketch of how persistence analysis for
LRU fully-associative caches~\cite{LRU_analysis_book, LRU_fix,
  LRU_ferdinand} can be extended when deterministic memory at the
cache controller is implemented according to
Algorithm~\ref{alg:cacherepl}. We indicate with ``DM-LRU'' the
resulting cache policy. In this section, we only discuss \emph{must}
analysis for the single-core case, to demonstrate that it is possible
to predict cache hits that could not be classified as \emph{always
  hit} for the same control flow (process) if DM was not
used. Following the outlined approach, \emph{may} analysis could also
be extended. Persistence analysis was first introduced
in~\cite{LRU_ali, LRU_ferdinand}, and formalized in~\cite{LRU_reineke,
  LRU_analysis_book}. We reuse some of the notation
in~\cite{LRU_analysis_book}, but due to space constraints we omit a
number of details.

In this analysis framework, \emph{must} analysis is performed by
considering abstracted cache states. \emph{Must} analysis keeps track
of the upper-bound on the age of each addressable memory block. The
abstract domain $DMLru_{D+B}$ is defined as $DMLru_{D+B} :=
\mathcal{B} \rightarrow \{0, \ldots, D-1\} \times \{D, \ldots, D+B-1,
\infty\}$, where $D+B = A$, with $A$ being the associativity of the
cache, and $D$ ($B$, resp.) is the number of lines marked as
deterministic (best-effort, resp.). An abstract state $q$ is then
represented as two sets of memory blocks $q =
[\{a,b\}],[\{c\},\{d\},\{e,f\}] \in DMLru_{D+B}$. In this example, we
have $D = 1, B = 3, A = 4$. Any block with DM-LRU age greater than or
equal to D is a best-effort block. Hence, blocks $a$ and $b$ are
deterministic lines, with maximum DM-LRU age 0. On the other hand $d$
is a best-effort block with maximum DM-LRU age 2.

%% When a new memory reference is performed, the access can lead to 4
%% different cases: ($M_d$) miss on DM line, ($H_d$) hit on DM line,
%% ($M_b$) miss on best-effort line, ($H_d$) hit on best-effort line.

The update abstract transformer $U_{D}$ for a deterministic memory
access $a$ can be defined as follows:

{\scriptsize
\begin{multline}
  U_{D}(q, a) := D' \leftarrow
  \begin{cases}
    D + 1 &:= D < A-1 \land q(a) \ge D\\
    D     &:= D = A \lor q(a) < D\\
  \end{cases},
  B' \leftarrow
  \begin{cases}
    B - 1 &:= D < A-1 \land q(a) \ge D\\
    B     &:= D = A \lor q(a) < D\\
  \end{cases},\\
  \lambda b. 
  \begin{cases}
    0         &:= b = a\\
    q(b)      &:= b \neq a \land q(b) < D \land q(b) \ge q(a) \\
    q(b)+1    &:= b \neq a \land q(b) < D \land q(b) < q(a) \land q(b) < D'-1\\
    \infty    &:= b \neq a \land q(b) < D \land q(b) < q(a) \land q(b) \ge D'-1\\
    q(b)      &:= b \neq a \land q(b) \ge D \land q(a) < D\\
    q(b)      &:= b \neq a \land q(b) \ge D \land q(b) \ge q(a)\\
    q(b)+1    &:= b \neq a \land q(b) \ge D \land q(b) < q(a) \land q(b) < A-1\\
    \infty    &:= b \neq a \land q(b) \ge D \land q(b) < q(a) \land q(b) \ge A-1\\
  \end{cases}
  \label{eq:u_d_transf}
\end{multline}
}

Where $D'$ ($B'$, resp.) is the new value of $D$ ($B$, resp.) after
the update. Similarly, the update abstract transformer $U_{B}$ for a
best-effort memory access $a$ can be defined as follows:

{\scriptsize
\begin{equation}
  U_{B}(q, a) :=
  \lambda b. 
  \begin{cases}
    D         &:= b = a\\
    q(b)      &:= b \neq a \land q(b) \ge q(a) \\
    q(b)+1    &:= b \neq a \land q(b) < q(a) \land q(b) < A-1\\
    \infty    &:= b \neq a \land q(b) < q(a) \land q(b) \ge A-1\\
  \end{cases}
\end{equation}
}

The join abstract transformer remains almost identical to what used in
traditional LRU \emph{must} analysis~\cite{LRU_reineke,
  LRU_analysis_book}: the joined state will contain only the blocks in
the intersection of the joining states, each with the maximum age in
any of the two states. The only difference is that $D$ is taken as the
maximum between the value of $D$ in the joining states. $B$ for the
new state is then computed as $A-D$.

To clarify update and join operations, consider the abstract state $q
= [\{a,b\}],[\{c\},\{d\},\{e,f\}]$, where $D = 1$.  Assume that
deterministic block $d$ is accessed, which is currently cached as
best-effort (this can happen after a context-switch). First, the value
of $D'$ ($B'$, resp.) is computed as $D' = D+1$ ($B' = B - 1$, resp.);
next, $\{a,b\}$ both satisfy the third condition in the age
transformation of $U_{D}$ (Equation~\ref{eq:u_d_transf}); block $c$
satisfies the seventh condition; $d$ the first; and $\{e,f\}$ the
sixth. The resulting updated abstract state is: $q' =
[\{d\},\{a,b\}],[\{c\},\{e,f\}]$. If we were to join $q$ with $q'$,
the resulting state would be $q'' = [\{\},\{a,b\}],[\{c,d\},\{e,f\}]$.

\begin{figure}
  \centering
  \includegraphics[width=.9\textwidth]{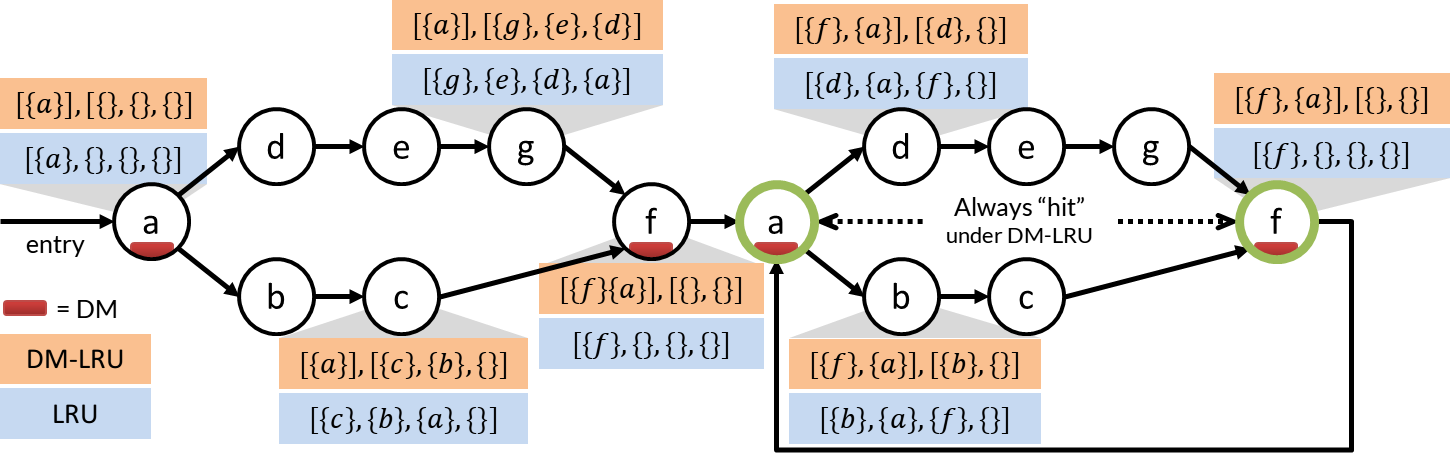}
  \caption{An example of \emph{must} analysis under DM-LRU (orange
    states), compared to traditional LRU (blue states). If $a$ and $f$
    are marked as DM, they can be classified as \emph{always hit} under
    DM-LRU.}
  \label{fig:dm_lru}
\end{figure}

We now demonstrate how this analysis can be applied to a simple
control-flow graph. The following example yields an important
conclusions: there exist instances where it is not possible to predict
any cache hit with traditional LRU, while under DM-LRU it is possible
to predict some cache hits. For our example, we consider a cache with
$A = 4$. The initial state is $[\{\},\{\},\{\},\{\}]$ and
$[~],[\{\},\{\},\{\},\{\}]$ for LRU and DM-LRU, respectively. The
progress of the analysis is depicted in Figure~\ref{fig:dm_lru}. As
shown in the example, blocks $a$ and $f$ can be classified as
\emph{persistent} (i.e. always hit after the first miss) under DM-LRU,
while they cannot be classified as \emph{always hit} if traditional LRU
is used.

\subsection{Overhead}
We now briefly discuss overhead of actual hardware implementation.
% DM-aware cache replacement algorithm overhead. this is in the
% critical path. right?
%% \fixme{Farzad. overhead of cache replacement algorithm (Algorithm 1)?}
% cache cleanup operation overhead
First, the space overhead of our approach is small: one bit storage
space per cache-line, which is less than 0.2\% for a standard 64 byte
cache-line space. The timing overhead of the deterministic
memory-aware cache replacement algorithm is not easy to analyze
without actual hardware implementation, but we conjecture it would
also be low because of the simplicity of our design and the fact that
cache replacement operations occur only at cache-misses which are
relatively less frequent operations.

One potentially costly operation 
is the deterministic memory cleanup operation, which requires updating
every cache line marked as deterministic (one bit per line) after the
corresponding task's context switch.
A simple hardware design would need to clear the DM bit of every
cache-line of a cache-partition one by one---until all cache lines of
the cache way partition are cleared. All accesses to the cache will be
blocked until the operation completes. 
%% In a multi-banked cache, each bank can be cleared in parallel to
%% reduce the total delay. Consider a 2MB, 8-bank,
%% 16-way set-associative cache, which is partitioned into four 4-way
%% partitions. Then each cache partition has up to 1k DM
%% bits/bank/partition to be cleared at each context switch. 
For a 2MB shared cache, the estimated time for it would be around one
$\mu$S, assuming bank-level parallelization.
Because the context switching occurs infrequently, we believe
this overhead is acceptable. The overhead can be further
reduced by using custom SRAM arrays that provide additional signal
lines, one per cache way, to clear all DM bit cells in the way. In
this case, the operation could be performed in few clock cycles.
